# Supplementary material for: dpBento: Benchmarking DPUs for Data Processing
Source: arXiv:2504.05536 source file (2025-04-07)
Supplement: Supplementary file 1 [file appendix.tex]

\section{appendix}

Appendix here.

%\end{appendix}
